# Supplementary material for: Sharp DNA denaturation in a helicoidal mesoscopic model
Source: arXiv:1910.07614 ancillary file (2020-05-25)
Supplement: Supplementary file 1 [file supplementary.pdf]

# Supplementary information: Sharp DNA denaturation in a helicoidal mesoscopic model

Mateus Rodrigues Leal Gerald Weber
Departamento de Física
Universidade Federal de Minas Gerais
31270-901 Belo Horizonte-MG, Brazil

21st May 2020

## S1 Numerical integrations

For all numerical calculations we used the Gauss-Legendre quadrature. The integration steps were 1500 for a fixed $b$, which is the most critical integration due to the occurrence of numerical instabilities and divergences. For the varying integration limit $b$ we used the rule of $200 + 60(b/\mathrm{nm})$ integration points. For $\zeta$ and $\Theta$, 10 integration points were found to be sufficient for achieving numerical convergence.

Eq. (8) expanded to second order of $\Delta z^2_{n,n-1}$

$$J_{n,n-1} \approx \Delta z_{n,n-1}\left[1+\frac{1}{2}\frac{f^2_{n,n-1}}{\Delta z^2_{n,n-1}}-\frac{1}{8}\left(\frac{f^2_{n,n-1}}{\Delta z^2_{n,n-1}}\right)^2\right] \tag{S1}$$

The equivalent of Eq. (12) is

$$\begin{aligned} Z_{r\theta z} &= \Gamma^N(2\zeta)^N \int_0^b \int_{-\Theta}^{\Theta} \prod_{n=1}^{N} d\theta_n r_n dr_n \exp\left[-\frac{\beta}{2}\left(V(r_n)+V(r_n)\right)\right] \\ &\times \exp\left[-\frac{\beta k}{8J_0^2}\left(f^4_{n,n-1}-\frac{f^6_{n,n-1}}{2J_0^2}+\frac{5f^8_{n,n-1}}{16J_0^4}\right)\right] \end{aligned} \tag{S2}$$

The equivalent of Eq. (14) is

$$\begin{aligned} Z^{app.}_{r\theta z} &= \Gamma^N(4\zeta\Theta)^N \int_0^b \prod_{n=1}^{N} dr_n\sqrt{r_n r_{n-1}} \exp\left\{-\frac{\beta}{2}\left[V(r_n)+V(r_n)\right]\right\} \\ &\times \exp\left\{-\frac{\beta k}{8J_0^2}\left[(r_n-r_{n-1})^2+\omega^2 r_n r_{n-1}\right]^2\right\} \\ &\times \exp\left\{\frac{\beta k}{16J_0^4}\left[(r_n-r_{n-1})^2+\omega^2 r_n r_{n-1}\right]^3\right\} \\ &\times \exp\left\{-\frac{5\beta k}{128J_0^6}\left[(r_n-r_{n-1})^2+\omega^2 r_n r_{n-1}\right]^4\right\} \end{aligned} \tag{S3}$$

And the kernel to second order, equivalent o Eq. (15), is

$$\begin{aligned} K(x,y) &= \sqrt{xy}\exp\left\{-\frac{\beta}{2}\left[V(x)+V(y)\right]\right\} \\ &\times \exp\left\{-\frac{\beta k}{8J_0^2}\left[(x-y)^2+\omega^2 xy\right]^2\right\} \\ &\times \exp\left\{\frac{\beta k}{16J_0^4}\left[(x-y)^2+\omega^2 xy\right]^3\right\} \\ &\times \exp\left\{-\frac{5\beta k}{128J_0^6}\left[(x-y)^2+\omega^2 xy\right]^4\right\} \end{aligned} \tag{S4}$$

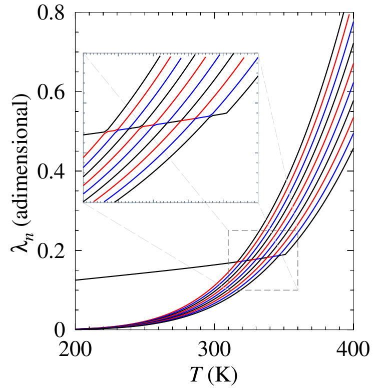


Figure S1: Equivalent to Fig. 2 for T2.

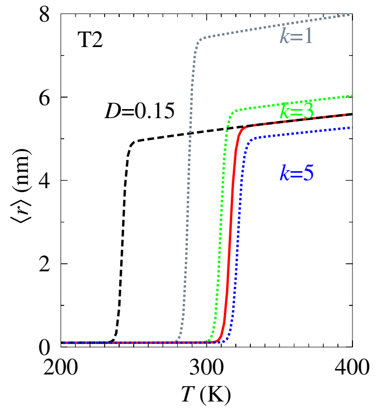


Figure S2: Equivalent to Fig. 3 for T2.
